# Supplementary material for: Suppression of the fieldlike spin-orbit torque efficiency due to the magnetic proximity effect in ferromagnet/platinum bilayers
Source: arXiv:1711.07969 ancillary file (2017-11-22)
Supplement: Supplementary file 1 [file supplemental.pdf]

## SUPPLEMENTAL INFORMATION

### Harmonic response measurement

To extract the dampinglike (DL) and fieldlike (FL) spin-orbit torque (SOT) effective magnetic fields $H_{DL}$ and $H_{FL}$ which appear in Eq. 1 in the main text, we used a harmonic response technique optimized for in-plane magnetized films. The technique follows closely from the original magnetoresistive (MR) harmonic response measurements of SOTs developed in References [1–3] for perpendicularly magnetized films, and the adaptation to in-plane magnetized films by Kawaguchi *et al.* [4]. Later, Avci *et al.* [5] discussed magnetothermoelectric (MTE) effects which must be accounted for in harmonic MR measurements of SOTs in the in-plane geometry. Our expressions are similar to Ref. [5], however we arrive at a more compact expression in a simplified geometry to account for MTE effects.

In the following, we describe our measurement details. Figure 1(a) shows a plan-view optical micrograph of an example Hall bar and description of the coordinate system used. The Hall bar width was 10 $\mu$m. A low-frequency ($\omega/2\pi \simeq 10$ Hz) ac excitation current $\sim \sin \omega t$ with root-mean-square (RMS) amplitude $I$ was applied to a Hall bar, and the second harmonic Hall resistance $R_H^{2\omega} \equiv \langle V_H^+ - V_H^- \rangle^{2\omega}/I$ was measured with phase and harmonic sensitive lock-in detection, where the brackets denote the RMS amplitude of the $2\omega$ Y-quadrature Hall voltage. The orientation $\phi$ of the static applied magnetic field $H$ was rotated 360° in the bilayer plane while recording $R_H^{2\omega}$, for varied magnetic field strengths. Figure 1(b-d) shows example data for different Pt thicknesses and temperature, where $H$ was varied between 0.6 T and 9 T. Below, we discuss the model that was used to fit the data and extract $H_{DL}$ and $H_{FL}$.

The DL and FL SOTs applied at $\omega$ give rise to $R_H^{2\omega}$ angular dependencies originating from the anomalous Hall effect (AHE) and planar Hall effect (PHE), respectively. The ac current results in an effective field $\boldsymbol{H}^\omega = H_{DL} \sin\phi \sin\omega t \hat{\boldsymbol{z}} + (H_{FL} + H_{Oe}) \sin\omega t \hat{\boldsymbol{y}}$, which tilts the magnetization small angles from the applied magnetic field at frequency $\omega$. The

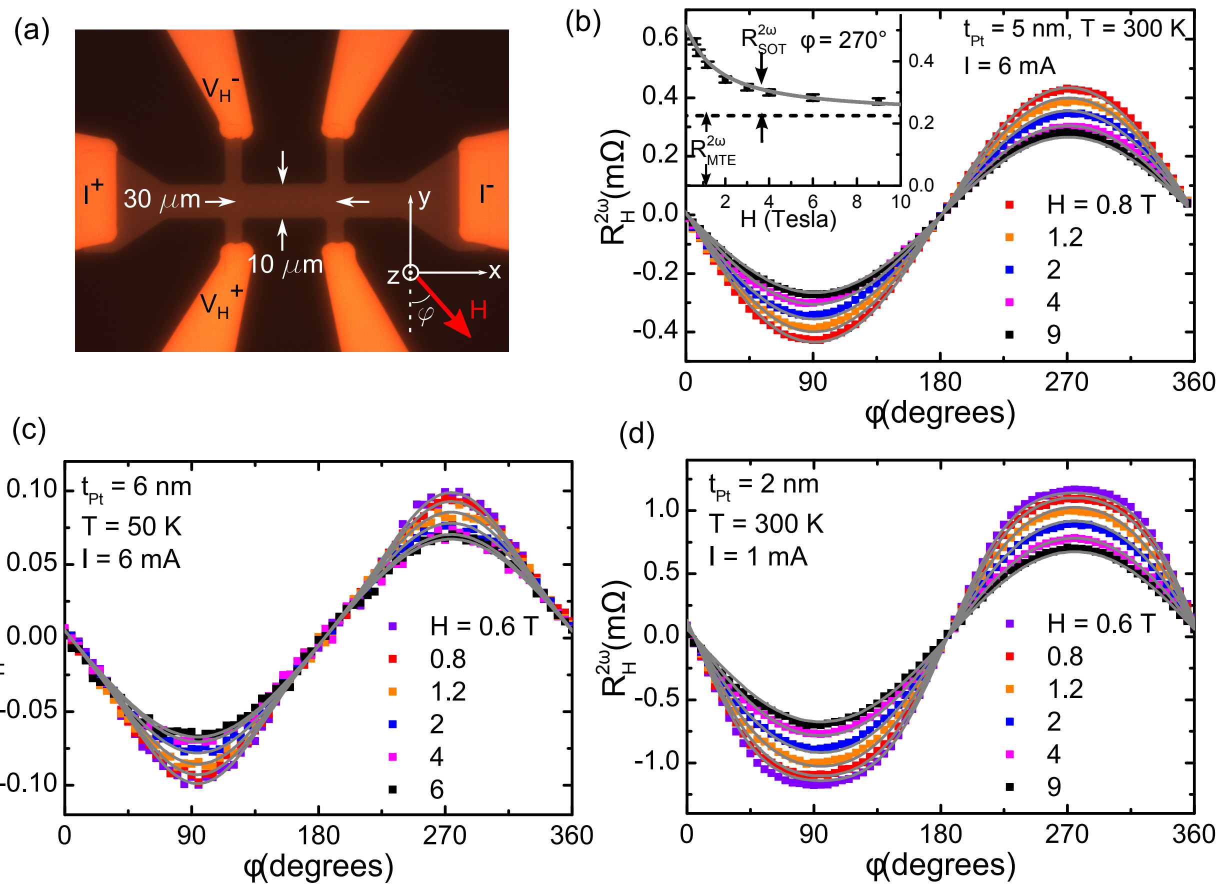


FIG. 1. (a) Plan view optical micrograph of an example Hall bar used in this study. The dimensions are indicated on the image, and the coordinate system is defined in the lower right. (b-d) Example second harmonic Hall resistance as function of in-plane angle $\phi$ for different applied magnetic fields, with the corresponding Pt thickness, temperature, and current indicated on the figure. The solid curves show the fit to Eq. 1. The angle-independent offset $R_0^{2\omega}$ was subtracted from the data shown. In (b), the fit values are $H_{DL} = 24$ Oe, $H_{FL} + H_{Oe} = -0.86$ Oe, and $R^{2\omega}_{MTE} = -0.22$ mΩ, in (c), $H_{DL} = 9.1$ Oe, $H_{FL} + H_{Oe} = -4.3$ Oe, and $R^{2\omega}_{MTE} = -0.059$ mΩ, and in (d), $H_{DL} = 12$ Oe, $H_{FL} + H_{Oe} = 2.9$ Oe, and $R^{2\omega}_{MTE} = -0.56$ mΩ. In the inset of (b), $R_H^{2\omega}$ at $\phi = 270°$ is plotted vs. magnetic field, with the fit to Eq. 1 shown as the solid curve. The dashed line indicates $R^{2\omega}_{\mathrm{MTE}}$.

AHE and PHE then result in a $2\omega$ Hall resistance given by [4, 5][6]

$$
\begin{aligned}
R_H^{2\omega}(\phi, H) = \\
& - \frac{1}{2}\frac{R_{AHE}H_{DL}}{(4\pi M_s + H)}\sin\phi \\
& - \frac{1}{2}\frac{R_{\text{PHE}}(H_{FL} + H_{Oe})}{H}(\sin 3\phi - \sin\phi) \\
& + R_{MTE}^{2\omega}\sin\phi + R_0^{2\omega},
\end{aligned}
\tag{1}
$$

where $R_{AHE}$ is the AHE resistance, $R_{PHE}$ is the PHE resistance, and $4\pi M_s$ is the out-of-plane demagnetization field. The $R_{MTE}^{2\omega}\sin\phi$ term captures MTE emfs such as the anomalous Nernst effect (ANE) and logitudinal spin-Seebeck effect (LSSE)[7–9], which go as $\nabla T \times \hat{\boldsymbol{m}}$. ($\nabla T$ is predominantly in the z-direction due to the flow of Joule heat into the substrate.) $R_0^{2\omega}$ is an overall offset that likely originates from the Seebeck effect due to small in-plane components of $\nabla T$. $H_{Oe}$ is the Oersted field that results from the ac excitation current in the Pt layer, and is calculated from Ampere's law. Equation 1 is valid for $H \gg H_{DL}, H_{FL}$. The applied magnetic field is much larger than the in-plane magnetic anisotropy field ($2K_1/M_s \simeq 150$ Oe at room temperature) such that the static magnetization may be considered saturated along the applied field direction at all $\phi$ angles for fields larger than a few kOe. The factors of $-1/2$ in the first and second terms in Eq. 1 arise from the trigonometric identity $\sin^2\omega t = (1/2)(1 - \cos 2\omega t)$, as the $2\omega$ lockin Y-quadrature signal is proportional to $\cos 2\omega t$. The AHE and PHE resistances were measured on the same Hall bar with low excitation current using conventional transport techniques for each Pt thickness and temperature. The sign of the SOT efficiency corresponds to the sign of the effective field (in a right-handed Cartesian coordinate system) produced by a charge current applied in the $+\hat{x}$ direction shown in Fig. 1(a). For example, the positive $\xi_{DL}$ values reflect $\boldsymbol{H}_{DL} \parallel +\hat{z}$ for $\hat{\boldsymbol{m}} \parallel +\hat{x}$, and the negative $\xi_{FL}$ values reflect $\boldsymbol{H}_{FL} \parallel -\hat{y}$ direction, both for current applied in $+\hat{x}$ direction. We verified that $H_{DL}$ and $H_{FL}$ increase linearly with excitation current, however current dependencies were not performed exhaustively as the $2\omega$ detection method itself guarantees that $R^{2\omega} \propto I$ (i.e. $V^{2\omega} \propto I^2$).

The 360° $\phi$-rotations at each Pt thickness and temperature were fit to Eq. 1 to extract $H_{DL}$ and $H_{FL}$, with a single set of fitting parameters ($H_{DL}$, $H_{FL}$, $R_{MTE}^{2\omega}$, and $R_0^{2\omega}$) used for all applied magnetic field strengths. The fits are compared to the example data in Fig. 1(b-d), showing Eq. 1 captured the measured data well. The $\sin\phi$-behavior of the data shown indicate that DL SOT and MTE effects dominate the angular dependence of $R_H^{2\omega}$,

while a smaller $\sin 3\phi - \sin\phi$ signal is present due to the sum of $H_{Oe}$ and $H_{FL}$. The more "triangular" shape of the Figure 1(c) data illustrate a case where $H_{FL} + H_{Oe} < 0$, and the more "square" shape of the Figure 1(d) data illustrate a case where $H_{FL} + H_{Oe} > 0$. In these bilayers, we observe MTE signals of comparable size to those due to SOT. The inset of Fig. 1(b) illustrates how the magnetic field dependence allows differentiation of the MTE signal from the DL SOT signal. We emphasize that for in-plane magnetized bilayers, the magnetic field dependence must be used to differentiate MTE $2\omega$ resistances from those due to the DL SOT.

The SOT effective magnetic fields $H_{DL}$ and $H_{FL}$ obtained by fitting as described above were input to Eq. 1 of the main text for each Pt thickness and temperature, resulting in the SOT efficiency data shown in Fig. 1(b) and Fig. 3 of the main text.

**Parallel resistances analysis used to extract resistivities**

In order to obtain the Pt resistivity and account for the shunted current distribution in the bilayer, the F and N layer were treated as parallel resistances. The sheet resistances $R_{xx}$ for each Pt thickness at 300 K and 20 K are shown in Fig. 1(a) of the main text. For ultrathin metal films the resistivity is well-approximated by the expression

$$\rho_{\mathrm{N}}(t_{\mathrm{N}}) = \rho_\infty + R_A/t_N, \tag{2}$$

where $\rho_\infty$ is the bulk ($t_N \to \infty$) resistivity, and $R_A$ is a surface resistance-area product that accounts for the increase in resistivity for thin films due to diffuse surface scattering[10]. Diffuse surface scattering dominates over grain boundary scattering in our films, as they are epitaxial. To account for the shunting effect of the 1.2 nm CFA layer, Eq. 2 was fit to the thickness dependence of $R_{xx}$ shown in Fig. 1(a) with a parallel-resistance model (i.e. $R_{xx}^{-1} = R_F^{-1} + R_N^{-1}$) and $R_F = \rho_F/t_F$, $\rho_\infty$, and $R_A$ as the fitting parameters. It was found that $\rho_F = 130\ \mu\Omega$cm, $\rho_\infty = 12\ \mu\Omega$cm, and $R_A = 88\ \mu\Omega$cm nm. The results of the fit are shown in the inset of Fig. 1(a) in the main text. The value of $\rho_\infty$ at 300 K we extract using this method is in good agreement with the 300 K resistivity reported for pure bulk Pt[11, 12]. Also $d\rho_\infty/dT = 0.038\ \mu\Omega$cm K$^{-1}$ in the 50-300 K temperature range, in good agreement with literature reports (0.037-0.040 $\mu\Omega$cm K$^{-1}$)[11, 12]. The current density in N, which is the $j_N^e$ factor in the denominator of Eq. 1 of the main text, is calculated using

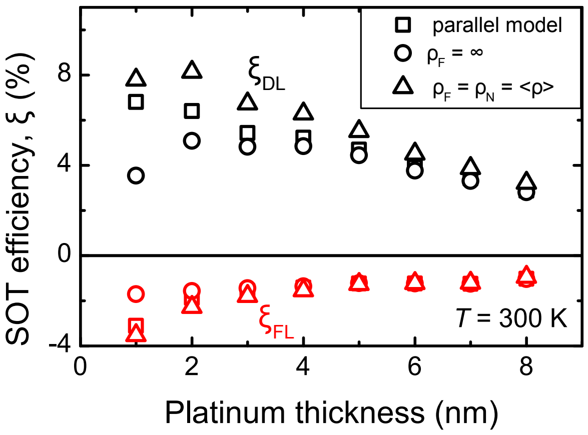


FIG. 2. Summary of the DL (black data) and FL (red data) SOT efficiencies at 300 K for various current shunting models. Shown as squares are the parallel resistance model values shown in the main text, the circles are obtained by setting $\rho_F = \infty$, and the triangles are for the uniform-resistivity model.

a standard current-divider expression

$$j_N^e = \frac{\sqrt{2}I}{t_N}\frac{R_F}{R_F + R_N} \tag{3}$$

where $R_N = \rho_N/t_N$, $R_F = \rho_F/t_F$, and the $\sqrt{2}$ in numerator converts $I$ from an RMS amplitude to a sinusoidal amplitude.

We briefly discuss possible systematic errors introduced by our method of treating the current shunting distribution in the bilayer. At small N thicknesses in all-metallic F/N bilayers, current shunting through the F layer represents the largest systematic error in calculating $\xi$. Approaches to account for current shunting in quantitative analysis vary: some have simply using a bilayer-averaged current density, and others have measured $\rho_F$ with a companion growth[13]. For example, in Fig. 2 we show how our measured SOT efficiencies are altered by assuming different possible shunting current distributions. In addition to the parallel resistance model described previously, in Fig. 2 we show SOT efficiencies obtained by setting $\rho_F = \infty$, and also with a uniform-resistivity assumption where $\rho_F = \rho_N = \langle\rho\rangle$. The latter case may be appropriate in the regime where the carrier mean free path is comparable to the bilayer thickness and the scattering is dominated by surface scattering, as is the case in our bilayers. However, the difference between the parallel resistance model used in the main text and the uniform resistivity model can be seen to be

small and does not change the results of the paper.

### Measurement of AHE and AMR resistances

Here we describe the measurement details used to measure $R_{AHE}$ and $R_{AMR}$, such as the values shown on Fig. 2 of the main text. Magnetic field sweeps over the range of $\pm$ 9 T were performed while recording $R_{xx}$ and $R_{xy}$, with the orientation of the magnetic field $H$ along the three coordinates $x, y$, and $z$ shown in Fig. 1(a). See Fig. 3 for example magnetic field sweeps. In Fig. 3(a), we indicate how the saturated-magnetization difference between $x$ and $z$ $H$-orientations gives $R_{AMR}$, which must be differentiated from spin-Hall magnetoresistance (SMR)[14–17] changes in resistance that occur between the $z$ and $y$ $H$-orientations. In Fig. 3(b) the $R_{xy}$ data are fit to the combined AHE and ordinary Hall effect (OHE) model to give $R_{AHE}$, which is the saturation value of the magnetization-dependent Hall resistance.

### Magnetoresistance including Pt shunting

The identification of the magnetic proximity effect (MPE) discussed in the main text relies on the differentiation of the observed magnetoresistance (MR) vs $R_{xx}$ behavior shown in Fig. 2 of the main text from that which would be expected if the MR originated from F shunting alone. In Fig. 2 of the main text, the data is visualized with temperature as an implicit variable. Here, in supplementary Fig. 4 we have included the same data plotted traditionally so that temperature is the explicit variable. To understand show the shorting effect of the N Pt layer influences the measured net MR, we first express the resistance tensors in both N and F as

$$R_F = \begin{bmatrix} R_{xx,F} & R_{xy,F} \\ -R_{xy,F} & R_{xx,F} \end{bmatrix}, R_N = \begin{bmatrix} R_{xx,N} & R_{xy,N} \\ -R_{xy,N} & R_{xx,N} \end{bmatrix}, \tag{4}$$

where we have enforced time-reversal symmetry ($R_{xy} = -R_{yx}$) and isotropic transport ($R_{xx} = R_{yy}$). The total resistance tensor $R_T$ is given by adding $R_F$ and $R_N$ in parallel, i.e. $R_T^{-1} = R_F^{-1} + R_N^{-1}$. To simplify we note that $R_{xx} \gg R_{xy}$ for both N and F, and for purpose of this exercise we take $R_{xy,N} = 0$. Carrying out the algebra and simplifying for the transverse

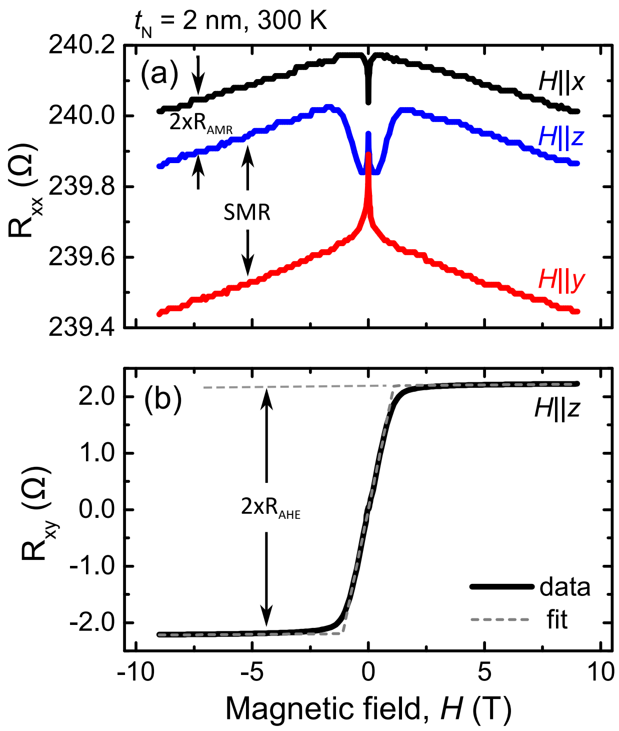


FIG. 3. Example ±9 T magnetic field sweeps for (a) $R_{xx}$ and (b) $R_{xy}$, which are used to extract $R_{AMR}$ and $R_{AHE}$ respectively as indicated on the figure. The orientation of the field is indicated on the figure where the coordinate system is defined in 1(a). In (b) the gray line shows the fit to piecewise defined OHE plus AHE resistance, which gives $R_{AHE} = 2.19\ \Omega$, AHE saturation field of 1.11 $T$, and OHE coefficient above saturation of $+1.4\pm\ 0.4\times10^{-11}\ m^3C^{-1}$. A small $H$-independent offset has been subtracted from the $R_{xy}$ data shown in (b), so that the data is odd with respect to $H$. All data shown in this figure was taken on the 2 nm Pt thickness at 300 K.

(i.e. Hall) total resistance we have

$$R_{xy,T} = \frac{R_{xx,N}^2 R_{xy,F}}{(R_{xx,F} + R_{xx,N})^2}. \tag{5}$$

In our case, $RRR_F \simeq 1$, so we may attribute all temperature dependence of $R_{xx,T}$ to temperature dependence of $R_{xx,N}$. To compare to the measured transverse resistance data, it is most helpful to rearrange Eq. 5 by substituting $R_{xx,N}^{-1} = R_{xx,T}^{-1} - R_{xx,F}^{-1}$. We then have

$$R_{xy,T} = \frac{R_{xx,T}^2 R_{xy,F}}{R_{xx,F}}, \tag{6}$$

therefore we expect $R_{xy,T} \propto R_{xx,T}^2$, for temperature-independent $R_{xy,F}, R_{xx,F}$. It is also straightforward to show for longitudinal MR (e.g. AMR) N shunting also gives rise to

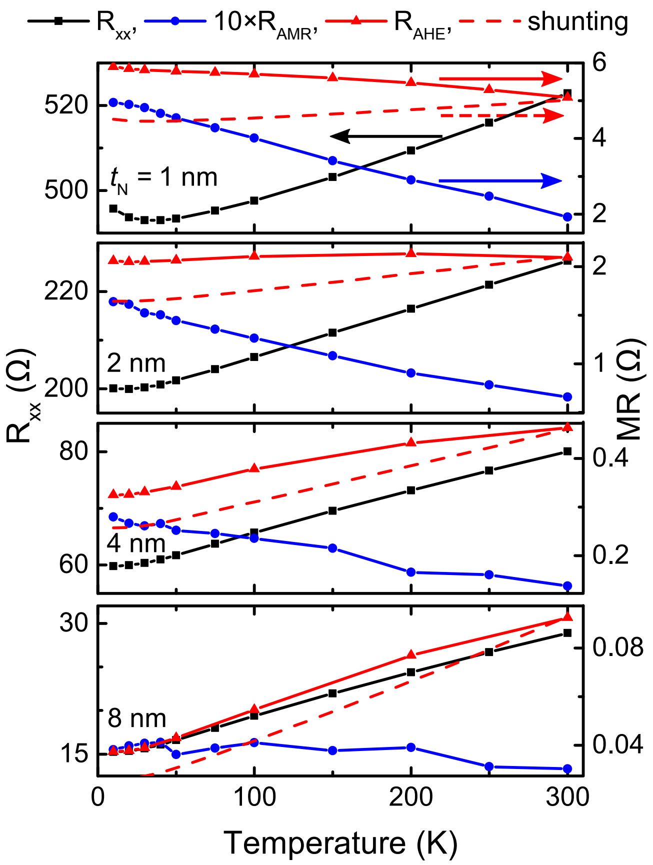


FIG. 4. The explicit temperature dependence of square resistance $R_{xx}$ (left ordinate, black squares), and MRs $R_{AHE}$ (right ordinate, red triangles) and $R_{AMR}$ (right ordinate, blue circles) for the 1, 2, 4, and 8 nm Pt thicknesses. $R_{AMR}$ has been multiplied by 10 for ease of visualization. The lines connect data points. Also shown as the dashed red line (right ordinate) is the F shunting prediction $R_{MR} \propto R_{xx}^2$, which has been scaled to match the 300 K $R_{AHE}$ value for ease of comparison. The data shown in this figure is the same as that shown in Fig. 2 of the main text, in which the temperature dependence is implicit.

$R_{AMR,T} \propto R_{xx,T}^2$. These expressions motivate the trendline drawn on Fig. 2 in the main text.

[1] U. H. Pi, K. Won Kim, J. Y. Bae, S. C. Lee, Y. J. Cho, K. S. Kim, and S. Seo, Applied Physics Letters **97**, 162507 (2010).

[2] J. Kim, J. Sinha, M. Hayashi, M. Yamanouchi, S. Fukami, T. Suzuki, S. Mitani, and H. Ohno, Nature Materials **12**, 240 (2012).

[3] S. Emori, U. Bauer, S.-M. Ahn, E. Martinez, and G. S. D. Beach, Nature Materials **12**, 611 (2013).

[4] M. Kawaguchi, K. Shimamura, S. Fukami, F. Matsukura, H. Ohno, T. Moriyama, D. Chiba, and T. Ono, Applied Physics Express **6**, 113002 (2013).

[5] C. O. Avci, K. Garello, M. Gabureac, A. Ghosh, A. Fuhrer, S. F. Alvarado, and P. Gambardella, Physical Review B **90**, 224427 (2014).

[6] The angle convention we use is shifted by 90° from that used in Refs. [4, 5]. Also, the $\sin 3\phi - \sin\phi$ term in Eq. 1 is identical to the angular dependence of the FL contribution used in Refs. [4, 5], however we have arrived at a more compact expression in the chosen geometry.

[7] S. Y. Huang, W. G. Wang, S. F. Lee, J. Kwo, and C. L. Chien, Physical Review Letters **107**, 216604 (2011).

[8] K. Uchida, M. Ishida, T. Kikkawa, A. Kirihara, T. Murakami, and E. Saitoh, Journal of Physics: Condensed Matter **26**, 343202 (2014).

[9] S. H. Wang, L. K. Zou, J. W. Cai, B. G. Shen, and J. R. Sun, Physical Review B **88**, 214304 (2013).

[10] E. H. Sondheimer, Advances in Physics **1** (1952).

[11] L. Abadlia, F. Gasser, K. Khalouk, M. Mayoufi, and J. G. Gasser, Review of Scientific Instruments **85**, 095121 (2014).

[12] D. R. Lide, "Handbook of Chemistry and Physics," (1996).

[13] M.-H. Nguyen, D. Ralph, and R. Buhrman, Physical Review Letters **116**, 126601 (2016).

[14] H. Nakayama, M. Althammer, Y.-T. Chen, K. Uchida, Y. Kajiwara, D. Kikuchi, T. Ohtani, S. Geprägs, M. Opel, S. Takahashi, R. Gross, G. E. W. Bauer, S. T. B. Goennenwein, and E. Saitoh, Physical Review Letters **110**, 206601 (2013).

[15] M. Althammer, S. Meyer, H. Nakayama, M. Schreier, S. Altmannshofer, M. Weiler, H. Huebl, S. Geprägs, M. Opel, R. Gross, D. Meier, C. Klewe, T. Kuschel, J.-M. Schmalhorst, G. Reiss, L. Shen, A. Gupta, Y.-T. Chen, G. E. W. Bauer, E. Saitoh, and S. T. B. Goennenwein, Physical Review B **87**, 224401 (2013).

[16] S. Meyer, M. Althammer, S. Geprägs, M. Opel, R. Gross, and S. T. B. Goennenwein, Applied Physics Letters **104** (2014), 10.1063/1.4885086.

[17] J. Kim, P. Sheng, S. Takahashi, S. Mitani, and M. Hayashi, Physical Review Letters **116**, 1 (2015).
